# Supplementary material for: Fairify: Fairness Verification of Neural Networks
Source: arXiv:2212.06140 source file (2022-12-14)
Supplement: Supplementary file 1 [file appendix.tex]

% \section{Appendix}
% \label{sec:appendix}

\begin{table*}[t]
      %\vspace{2mm}
      \centering
      % \footnotesize
      % \setlength\tabcolsep{1.5pt}
      \caption{Extended fairness verification results (supplementary to Table 2 in the paper).
      Experiment setup: soft-timeout 100s, hard-timeout 30m, max-partition size: 100 (BM, GC), 10 (AC). BL: Baseline (w/ P - with Partitioning), Ver: Verification, \#P: number of partitions, Cov: Coverage, US: UNSAT, UNK: UNKNOWN \#H-At: number of times heuristic pruning attempted, C: average \textbf{c}ompression ratio -- (S): sound pruning, (H): heuristic pruning, Average time (second) {\tiny\VarClock} -- SV: sound verification, HV: heuristic verification.}
        \begin{tabular}{|c|l|ll|l|rrrrrrrrrrrr|}
        \hline
        \rowcolor[rgb]{ .851,  .851,  .851} \multicolumn{1}{|l|}{\textbf{PA}} & \textbf{Model} & \textbf{BL} & \textbf{B w/ P} & \textbf{Ver} & \multicolumn{1}{l}{\textbf{\#P}} & \multicolumn{1}{l}{\textbf{Cov \%}} & \multicolumn{1}{l}{\textbf{SAT}} & \multicolumn{1}{l}{\textbf{US}} & \multicolumn{1}{l}{\textbf{UNK}} & \multicolumn{1}{l}{\textbf{\#H}} & \multicolumn{1}{l}{\textbf{\#HS}} & \multicolumn{1}{l}{\textbf{C(S)}} & \multicolumn{1}{l}{\textbf{C(H)}} & \multicolumn{1}{l}{\textbf{SV {\tiny\VarClock}}} & \multicolumn{1}{l}{\textbf{HV {\tiny\VarClock}}} & \multicolumn{1}{l|}{\textbf{Total {\tiny\VarClock}}} \\
        \hline
        \multirow{8}[2]{*}{\begin{sideways}Age\end{sideways}} & BM1   & UNK   & UNK   & SAT   & 75    & 13.14 & 9     & 58    & 8     & 9     & 1     & 0.90  & 0.01  & 14.04 & 11.00 & 25.40 \\
              & \cellcolor[rgb]{ .949,  .949,  .949}BM2 & \cellcolor[rgb]{ .949,  .949,  .949}UNK & \cellcolor[rgb]{ .949,  .949,  .949}UNK & \cellcolor[rgb]{ .949,  .949,  .949}SAT & \cellcolor[rgb]{ .949,  .949,  .949}141 & \cellcolor[rgb]{ .949,  .949,  .949}26.08 & \cellcolor[rgb]{ .949,  .949,  .949}30 & \cellcolor[rgb]{ .949,  .949,  .949}103 & \cellcolor[rgb]{ .949,  .949,  .949}8 & \cellcolor[rgb]{ .949,  .949,  .949}9 & \cellcolor[rgb]{ .949,  .949,  .949}1 & \cellcolor[rgb]{ .949,  .949,  .949}0.85 & \cellcolor[rgb]{ .949,  .949,  .949}0.01 & \cellcolor[rgb]{ .949,  .949,  .949}7.76 & \cellcolor[rgb]{ .949,  .949,  .949}5.83 & \cellcolor[rgb]{ .949,  .949,  .949}13.84 \\
              & BM3   & UNK   & UNK   & SAT   & 139   & 26.47 & 27    & 108   & 4     & 6     & 2     & 0.96  & 0.00  & 9.78  & 3.42  & 13.49 \\
              & \cellcolor[rgb]{ .949,  .949,  .949}BM4 & \cellcolor[rgb]{ .949,  .949,  .949}UNK & \cellcolor[rgb]{ .949,  .949,  .949}UNK & \cellcolor[rgb]{ .949,  .949,  .949}SAT & \cellcolor[rgb]{ .949,  .949,  .949}37 & \cellcolor[rgb]{ .949,  .949,  .949}6.08 & \cellcolor[rgb]{ .949,  .949,  .949}1 & \cellcolor[rgb]{ .949,  .949,  .949}30 & \cellcolor[rgb]{ .949,  .949,  .949}6 & \cellcolor[rgb]{ .949,  .949,  .949}6 & \cellcolor[rgb]{ .949,  .949,  .949}0 & \cellcolor[rgb]{ .949,  .949,  .949}0.91 & \cellcolor[rgb]{ .949,  .949,  .949}0.03 & \cellcolor[rgb]{ .949,  .949,  .949}17.10 & \cellcolor[rgb]{ .949,  .949,  .949}16.29 & \cellcolor[rgb]{ .949,  .949,  .949}49.98 \\
              & BM5   & UNK   & UNK   & SAT   & 510   & 99.61 & 114   & 394   & 2     & 7     & 5     & 0.83  & 0.00  & 2.29  & 0.54  & 2.96 \\
              & \cellcolor[rgb]{ .949,  .949,  .949}BM6 & \cellcolor[rgb]{ .949,  .949,  .949}UNK & \cellcolor[rgb]{ .949,  .949,  .949}UNK & \cellcolor[rgb]{ .949,  .949,  .949}SAT & \cellcolor[rgb]{ .949,  .949,  .949}510 & \cellcolor[rgb]{ .949,  .949,  .949}100.00 & \cellcolor[rgb]{ .949,  .949,  .949}156 & \cellcolor[rgb]{ .949,  .949,  .949}354 & \cellcolor[rgb]{ .949,  .949,  .949}0 & \cellcolor[rgb]{ .949,  .949,  .949}3 & \cellcolor[rgb]{ .949,  .949,  .949}3 & \cellcolor[rgb]{ .949,  .949,  .949}0.76 & \cellcolor[rgb]{ .949,  .949,  .949}0.00 & \cellcolor[rgb]{ .949,  .949,  .949}1.17 & \cellcolor[rgb]{ .949,  .949,  .949}0.08 & \cellcolor[rgb]{ .949,  .949,  .949}1.36 \\
              & BM7   & UNK   & UNK   & SAT   & 124   & 23.33 & 62    & 57    & 5     & 9     & 4     & 0.92  & 0.01  & 8.31  & 5.10  & 14.89 \\
              & \cellcolor[rgb]{ .949,  .949,  .949}BM8 & \cellcolor[rgb]{ .949,  .949,  .949}UNK & \cellcolor[rgb]{ .949,  .949,  .949}UNK & \cellcolor[rgb]{ .949,  .949,  .949}SAT & \cellcolor[rgb]{ .949,  .949,  .949}23 & \cellcolor[rgb]{ .949,  .949,  .949}3.14 & \cellcolor[rgb]{ .949,  .949,  .949}1 & \cellcolor[rgb]{ .949,  .949,  .949}15 & \cellcolor[rgb]{ .949,  .949,  .949}7 & \cellcolor[rgb]{ .949,  .949,  .949}10 & \cellcolor[rgb]{ .949,  .949,  .949}3 & \cellcolor[rgb]{ .949,  .949,  .949}0.79 & \cellcolor[rgb]{ .949,  .949,  .949}0.04 & \cellcolor[rgb]{ .949,  .949,  .949}46.23 & \cellcolor[rgb]{ .949,  .949,  .949}31.64 & \cellcolor[rgb]{ .949,  .949,  .949}79.08 \\
        \hline
        \hline
        \multirow{5}[2]{*}{\begin{sideways}Sex\end{sideways}} & GC1   & UNK   & UNK   & SAT   & 31    & 13.43 & 27    & 0     & 4     & 6     & 2     & 0.76  & 0.01  & 41.78 & 15.98 & 58.18 \\
              & \cellcolor[rgb]{ .949,  .949,  .949}GC2 & \cellcolor[rgb]{ .949,  .949,  .949}UNK & \cellcolor[rgb]{ .949,  .949,  .949}UNK & \cellcolor[rgb]{ .949,  .949,  .949}SAT & \cellcolor[rgb]{ .949,  .949,  .949}11 & \cellcolor[rgb]{ .949,  .949,  .949}1.99 & \cellcolor[rgb]{ .949,  .949,  .949}4 & \cellcolor[rgb]{ .949,  .949,  .949}0 & \cellcolor[rgb]{ .949,  .949,  .949}7 & \cellcolor[rgb]{ .949,  .949,  .949}9 & \cellcolor[rgb]{ .949,  .949,  .949}2 & \cellcolor[rgb]{ .949,  .949,  .949}0.78 & \cellcolor[rgb]{ .949,  .949,  .949}0.04 & \cellcolor[rgb]{ .949,  .949,  .949}97.18 & \cellcolor[rgb]{ .949,  .949,  .949}75.67 & \cellcolor[rgb]{ .949,  .949,  .949}174.18 \\
              & GC3   & UNK   & UNK   & SAT   & 201   & 100.00 & 195   & 6     & 0     & 1     & 1     & 0.69  & 0.00  & 1.29  & 0.24  & 1.63 \\
              & \cellcolor[rgb]{ .949,  .949,  .949}GC4 & \cellcolor[rgb]{ .949,  .949,  .949}UNK & \cellcolor[rgb]{ .949,  .949,  .949}UNK & \cellcolor[rgb]{ .949,  .949,  .949}SAT & \cellcolor[rgb]{ .949,  .949,  .949}201 & \cellcolor[rgb]{ .949,  .949,  .949}100.00 & \cellcolor[rgb]{ .949,  .949,  .949}2 & \cellcolor[rgb]{ .949,  .949,  .949}199 & \cellcolor[rgb]{ .949,  .949,  .949}0 & \cellcolor[rgb]{ .949,  .949,  .949}1 & \cellcolor[rgb]{ .949,  .949,  .949}1 & \cellcolor[rgb]{ .949,  .949,  .949}0.63 & \cellcolor[rgb]{ .949,  .949,  .949}0.00 & \cellcolor[rgb]{ .949,  .949,  .949}0.73 & \cellcolor[rgb]{ .949,  .949,  .949}0.14 & \cellcolor[rgb]{ .949,  .949,  .949}0.97 \\
              & GC5   & UNK   & UNK   & UNK   & 12    & 1.49  & 0     & 3     & 9     & 9     & 0     & 0.59  & 0.03  & 75.27 & 75.43 & 151.53 \\
        \hline
        \multirow{5}[2]{*}{\begin{sideways}Age\end{sideways}} & \cellcolor[rgb]{ .949,  .949,  .949}GC1 & \cellcolor[rgb]{ .949,  .949,  .949}UNK & \cellcolor[rgb]{ .949,  .949,  .949}UNK & \cellcolor[rgb]{ .949,  .949,  .949}SAT & \cellcolor[rgb]{ .949,  .949,  .949}46 & \cellcolor[rgb]{ .949,  .949,  .949}20.40 & \cellcolor[rgb]{ .949,  .949,  .949}41 & \cellcolor[rgb]{ .949,  .949,  .949}0 & \cellcolor[rgb]{ .949,  .949,  .949}5 & \cellcolor[rgb]{ .949,  .949,  .949}8 & \cellcolor[rgb]{ .949,  .949,  .949}3 & \cellcolor[rgb]{ .949,  .949,  .949}0.75 & \cellcolor[rgb]{ .949,  .949,  .949}0.01 & \cellcolor[rgb]{ .949,  .949,  .949}29.72 & \cellcolor[rgb]{ .949,  .949,  .949}12.96 & \cellcolor[rgb]{ .949,  .949,  .949}43.19 \\
              & GC2   & UNK   & UNK   & SAT   & 13    & 3.98  & 8     & 0     & 5     & 10    & 5     & 0.82  & 0.04  & 88.11 & 52.42 & 141.86 \\
              & \cellcolor[rgb]{ .949,  .949,  .949}GC3 & \cellcolor[rgb]{ .949,  .949,  .949}UNK & \cellcolor[rgb]{ .949,  .949,  .949}UNK & \cellcolor[rgb]{ .949,  .949,  .949}SAT & \cellcolor[rgb]{ .949,  .949,  .949}201 & \cellcolor[rgb]{ .949,  .949,  .949}100.00 & \cellcolor[rgb]{ .949,  .949,  .949}195 & \cellcolor[rgb]{ .949,  .949,  .949}6 & \cellcolor[rgb]{ .949,  .949,  .949}0 & \cellcolor[rgb]{ .949,  .949,  .949}1 & \cellcolor[rgb]{ .949,  .949,  .949}1 & \cellcolor[rgb]{ .949,  .949,  .949}0.69 & \cellcolor[rgb]{ .949,  .949,  .949}0.00 & \cellcolor[rgb]{ .949,  .949,  .949}1.41 & \cellcolor[rgb]{ .949,  .949,  .949}0.22 & \cellcolor[rgb]{ .949,  .949,  .949}1.74 \\
              & GC4   & UNK   & UNK   & SAT   & 201   & 100.00 & 2     & 199   & 0     & 1     & 1     & 0.63  & 0.00  & 0.73  & 0.16  & 1.00 \\
              & \cellcolor[rgb]{ .949,  .949,  .949}GC5 & \cellcolor[rgb]{ .949,  .949,  .949}UNK & \cellcolor[rgb]{ .949,  .949,  .949}UNK & \cellcolor[rgb]{ .949,  .949,  .949}UNK & \cellcolor[rgb]{ .949,  .949,  .949}13 & \cellcolor[rgb]{ .949,  .949,  .949}1.99 & \cellcolor[rgb]{ .949,  .949,  .949}0 & \cellcolor[rgb]{ .949,  .949,  .949}4 & \cellcolor[rgb]{ .949,  .949,  .949}9 & \cellcolor[rgb]{ .949,  .949,  .949}9 & \cellcolor[rgb]{ .949,  .949,  .949}0 & \cellcolor[rgb]{ .949,  .949,  .949}0.62 & \cellcolor[rgb]{ .949,  .949,  .949}0.03 & \cellcolor[rgb]{ .949,  .949,  .949}69.49 & \cellcolor[rgb]{ .949,  .949,  .949}69.73 & \cellcolor[rgb]{ .949,  .949,  .949}139.73 \\
        \hline
        \hline
        \multirow{12}[2]{*}{\begin{sideways}Race\end{sideways}} & AC1   & UNK   & UNK   & SAT   & 29    & 0.14  & 8     & 15    & 6     & 8     & 2     & 0.64  & 0.04  & 40.73 & 23.50 & 64.43 \\
              & \cellcolor[rgb]{ .949,  .949,  .949}AC2 & \cellcolor[rgb]{ .949,  .949,  .949}UNK & \cellcolor[rgb]{ .949,  .949,  .949}UNK & \cellcolor[rgb]{ .949,  .949,  .949}SAT & \cellcolor[rgb]{ .949,  .949,  .949}15 & \cellcolor[rgb]{ .949,  .949,  .949}0.04 & \cellcolor[rgb]{ .949,  .949,  .949}4 & \cellcolor[rgb]{ .949,  .949,  .949}3 & \cellcolor[rgb]{ .949,  .949,  .949}8 & \cellcolor[rgb]{ .949,  .949,  .949}10 & \cellcolor[rgb]{ .949,  .949,  .949}2 & \cellcolor[rgb]{ .949,  .949,  .949}0.82 & \cellcolor[rgb]{ .949,  .949,  .949}0.04 & \cellcolor[rgb]{ .949,  .949,  .949}72.62 & \cellcolor[rgb]{ .949,  .949,  .949}54.86 & \cellcolor[rgb]{ .949,  .949,  .949}128.45 \\
              & AC3   & UNK   & UNK   & SAT   & 23    & 0.11  & 16    & 1     & 6     & 10    & 4     & 0.75  & 0.02  & 52.75 & 32.33 & 85.40 \\
              & \cellcolor[rgb]{ .949,  .949,  .949}AC4 & \cellcolor[rgb]{ .949,  .949,  .949}UNK & \cellcolor[rgb]{ .949,  .949,  .949}UNK & \cellcolor[rgb]{ .949,  .949,  .949}UNK & \cellcolor[rgb]{ .949,  .949,  .949}8 & \cellcolor[rgb]{ .949,  .949,  .949}0.00 & \cellcolor[rgb]{ .949,  .949,  .949}0 & \cellcolor[rgb]{ .949,  .949,  .949}0 & \cellcolor[rgb]{ .949,  .949,  .949}8 & \cellcolor[rgb]{ .949,  .949,  .949}8 & \cellcolor[rgb]{ .949,  .949,  .949}0 & \cellcolor[rgb]{ .949,  .949,  .949}0.67 & \cellcolor[rgb]{ .949,  .949,  .949}0.20 & \cellcolor[rgb]{ .949,  .949,  .949}100.57 & \cellcolor[rgb]{ .949,  .949,  .949}100.08 & \cellcolor[rgb]{ .949,  .949,  .949}241.70 \\
              & AC5   & UNK   & UNK   & SAT   & 10    & 0.02  & 3     & 0     & 7     & 9     & 2     & 0.71  & 0.13  & 98.14 & 74.06 & 180.41 \\
              & \cellcolor[rgb]{ .949,  .949,  .949}AC6 & \cellcolor[rgb]{ .949,  .949,  .949}SAT & \cellcolor[rgb]{ .949,  .949,  .949}SAT & \cellcolor[rgb]{ .949,  .949,  .949}SAT & \cellcolor[rgb]{ .949,  .949,  .949}19 & \cellcolor[rgb]{ .949,  .949,  .949}0.07 & \cellcolor[rgb]{ .949,  .949,  .949}6 & \cellcolor[rgb]{ .949,  .949,  .949}5 & \cellcolor[rgb]{ .949,  .949,  .949}8 & \cellcolor[rgb]{ .949,  .949,  .949}9 & \cellcolor[rgb]{ .949,  .949,  .949}1 & \cellcolor[rgb]{ .949,  .949,  .949}0.49 & \cellcolor[rgb]{ .949,  .949,  .949}0.05 & \cellcolor[rgb]{ .949,  .949,  .949}55.70 & \cellcolor[rgb]{ .949,  .949,  .949}44.43 & \cellcolor[rgb]{ .949,  .949,  .949}100.37 \\
              & AC7   & UNK   & UNK   & UNK   & 14    & 0.04  & 0     & 7     & 7     & 10    & 3     & 0.59  & 0.11  & 78.22 & 51.09 & 132.28 \\
              & \cellcolor[rgb]{ .949,  .949,  .949}AC8 & \cellcolor[rgb]{ .949,  .949,  .949}UNK & \cellcolor[rgb]{ .949,  .949,  .949}UNK & \cellcolor[rgb]{ .949,  .949,  .949}SAT & \cellcolor[rgb]{ .949,  .949,  .949}101 & \cellcolor[rgb]{ .949,  .949,  .949}0.63 & \cellcolor[rgb]{ .949,  .949,  .949}82 & \cellcolor[rgb]{ .949,  .949,  .949}19 & \cellcolor[rgb]{ .949,  .949,  .949}0 & \cellcolor[rgb]{ .949,  .949,  .949}1 & \cellcolor[rgb]{ .949,  .949,  .949}1 & \cellcolor[rgb]{ .949,  .949,  .949}0.22 & \cellcolor[rgb]{ .949,  .949,  .949}0.00 & \cellcolor[rgb]{ .949,  .949,  .949}17.59 & \cellcolor[rgb]{ .949,  .949,  .949}0.13 & \cellcolor[rgb]{ .949,  .949,  .949}17.84 \\
              & AC9   & UNK      & UNK      & SAT   & 741   & 4.63  & 399   & 342   & 0     & 4     & 4     & 0.19  & 0.00  & 2.29  & 0.02  & 2.44 \\
              & \cellcolor[rgb]{ .949,  .949,  .949}AC10 & \cellcolor[rgb]{ .949,  .949,  .949}UNK & \cellcolor[rgb]{ .949,  .949,  .949}UNK & \cellcolor[rgb]{ .949,  .949,  .949}SAT & \cellcolor[rgb]{ .949,  .949,  .949}20 & \cellcolor[rgb]{ .949,  .949,  .949}0.09 & \cellcolor[rgb]{ .949,  .949,  .949}6 & \cellcolor[rgb]{ .949,  .949,  .949}8 & \cellcolor[rgb]{ .949,  .949,  .949}6 & \cellcolor[rgb]{ .949,  .949,  .949}10 & \cellcolor[rgb]{ .949,  .949,  .949}4 & \cellcolor[rgb]{ .949,  .949,  .949}0.27 & \cellcolor[rgb]{ .949,  .949,  .949}0.05 & \cellcolor[rgb]{ .949,  .949,  .949}62.07 & \cellcolor[rgb]{ .949,  .949,  .949}32.82 & \cellcolor[rgb]{ .949,  .949,  .949}95.07 \\
              & AC11  & UNK   & UNK   & UNK   & 9     & 0.00  & 0     & 0     & 9     & 9     & 0     & 0.11  & 0.02  & 100.13 & 100.12 & 200.66 \\
              & \cellcolor[rgb]{ .949,  .949,  .949}AC12 & \cellcolor[rgb]{ .949,  .949,  .949}UNK & \cellcolor[rgb]{ .949,  .949,  .949}UNK & \cellcolor[rgb]{ .949,  .949,  .949}UNK & \cellcolor[rgb]{ .949,  .949,  .949}16 & \cellcolor[rgb]{ .949,  .949,  .949}0.04 & \cellcolor[rgb]{ .949,  .949,  .949}0 & \cellcolor[rgb]{ .949,  .949,  .949}7 & \cellcolor[rgb]{ .949,  .949,  .949}9 & \cellcolor[rgb]{ .949,  .949,  .949}9 & \cellcolor[rgb]{ .949,  .949,  .949}0 & \cellcolor[rgb]{ .949,  .949,  .949}0.29 & \cellcolor[rgb]{ .949,  .949,  .949}0.01 & \cellcolor[rgb]{ .949,  .949,  .949}57.56 & \cellcolor[rgb]{ .949,  .949,  .949}56.35 & \cellcolor[rgb]{ .949,  .949,  .949}114.19 \\
        \hline
        \multirow{12}[2]{*}{\begin{sideways}Sex\end{sideways}} & AC1   & UNK   & UNK   & SAT   & 24    & 0.11  & 4     & 13    & 7     & 10    & 3     & 0.65  & 0.06  & 43.46 & 32.52 & 76.18 \\
              & \cellcolor[rgb]{ .949,  .949,  .949}AC2 & \cellcolor[rgb]{ .949,  .949,  .949}UNK & \cellcolor[rgb]{ .949,  .949,  .949}UNK & \cellcolor[rgb]{ .949,  .949,  .949}SAT & \cellcolor[rgb]{ .949,  .949,  .949}17 & \cellcolor[rgb]{ .949,  .949,  .949}0.07 & \cellcolor[rgb]{ .949,  .949,  .949}3 & \cellcolor[rgb]{ .949,  .949,  .949}8 & \cellcolor[rgb]{ .949,  .949,  .949}6 & \cellcolor[rgb]{ .949,  .949,  .949}8 & \cellcolor[rgb]{ .949,  .949,  .949}2 & \cellcolor[rgb]{ .949,  .949,  .949}0.83 & \cellcolor[rgb]{ .949,  .949,  .949}0.02 & \cellcolor[rgb]{ .949,  .949,  .949}63.50 & \cellcolor[rgb]{ .949,  .949,  .949}41.78 & \cellcolor[rgb]{ .949,  .949,  .949}106.05 \\
              & AC3   & UNK   & UNK   & SAT   & 31    & 0.17  & 27    & 0     & 4     & 8     & 4     & 0.75  & 0.02  & 44.63 & 16.76 & 61.72 \\
              & \cellcolor[rgb]{ .949,  .949,  .949}AC4 & \cellcolor[rgb]{ .949,  .949,  .949}UNK & \cellcolor[rgb]{ .949,  .949,  .949}UNK & \cellcolor[rgb]{ .949,  .949,  .949}SAT & \cellcolor[rgb]{ .949,  .949,  .949}9 & \cellcolor[rgb]{ .949,  .949,  .949}0.01 & \cellcolor[rgb]{ .949,  .949,  .949}2 & \cellcolor[rgb]{ .949,  .949,  .949}0 & \cellcolor[rgb]{ .949,  .949,  .949}7 & \cellcolor[rgb]{ .949,  .949,  .949}8 & \cellcolor[rgb]{ .949,  .949,  .949}1 & \cellcolor[rgb]{ .949,  .949,  .949}0.78 & \cellcolor[rgb]{ .949,  .949,  .949}0.10 & \cellcolor[rgb]{ .949,  .949,  .949}98.98 & \cellcolor[rgb]{ .949,  .949,  .949}82.21 & \cellcolor[rgb]{ .949,  .949,  .949}205.17 \\
              & AC5   & UNK   & UNK   & SAT   & 9     & 0.00  & 0     & 0     & 9     & 9     & 0     & 0.77  & 0.09  & 100.20 & 100.11 & 205.50 \\
              & \cellcolor[rgb]{ .949,  .949,  .949}AC6 & \cellcolor[rgb]{ .949,  .949,  .949}UNK & \cellcolor[rgb]{ .949,  .949,  .949}UNK & \cellcolor[rgb]{ .949,  .949,  .949}SAT & \cellcolor[rgb]{ .949,  .949,  .949}22 & \cellcolor[rgb]{ .949,  .949,  .949}0.09 & \cellcolor[rgb]{ .949,  .949,  .949}8 & \cellcolor[rgb]{ .949,  .949,  .949}6 & \cellcolor[rgb]{ .949,  .949,  .949}8 & \cellcolor[rgb]{ .949,  .949,  .949}10 & \cellcolor[rgb]{ .949,  .949,  .949}2 & \cellcolor[rgb]{ .949,  .949,  .949}0.57 & \cellcolor[rgb]{ .949,  .949,  .949}0.05 & \cellcolor[rgb]{ .949,  .949,  .949}46.65 & \cellcolor[rgb]{ .949,  .949,  .949}39.40 & \cellcolor[rgb]{ .949,  .949,  .949}86.26 \\
              & AC7   & UNK   & UNK   & UNK   & 13    & 0.04  & 0     & 7     & 6     & 11    & 5     & 0.63  & 0.08  & 86.51 & 52.15 & 141.19 \\
              & \cellcolor[rgb]{ .949,  .949,  .949}AC8 & \cellcolor[rgb]{ .949,  .949,  .949}UNK & \cellcolor[rgb]{ .949,  .949,  .949}UNK & \cellcolor[rgb]{ .949,  .949,  .949}SAT & \cellcolor[rgb]{ .949,  .949,  .949}103 & \cellcolor[rgb]{ .949,  .949,  .949}0.64 & \cellcolor[rgb]{ .949,  .949,  .949}80 & \cellcolor[rgb]{ .949,  .949,  .949}23 & \cellcolor[rgb]{ .949,  .949,  .949}0 & \cellcolor[rgb]{ .949,  .949,  .949}2 & \cellcolor[rgb]{ .949,  .949,  .949}2 & \cellcolor[rgb]{ .949,  .949,  .949}0.24 & \cellcolor[rgb]{ .949,  .949,  .949}0.00 & \cellcolor[rgb]{ .949,  .949,  .949}16.99 & \cellcolor[rgb]{ .949,  .949,  .949}0.42 & \cellcolor[rgb]{ .949,  .949,  .949}17.53 \\
              & AC9   & UNK      & UNK      & SAT   & 332   & 2.08  & 161   & 171   & 0     & 1     & 1     & 0.20  & 0.00  & 5.28  & 0.17  & 5.56 \\
              & \cellcolor[rgb]{ .949,  .949,  .949}AC10 & \cellcolor[rgb]{ .949,  .949,  .949}UNK & \cellcolor[rgb]{ .949,  .949,  .949}UNK & \cellcolor[rgb]{ .949,  .949,  .949}SAT & \cellcolor[rgb]{ .949,  .949,  .949}31 & \cellcolor[rgb]{ .949,  .949,  .949}0.18 & \cellcolor[rgb]{ .949,  .949,  .949}10 & \cellcolor[rgb]{ .949,  .949,  .949}18 & \cellcolor[rgb]{ .949,  .949,  .949}3 & \cellcolor[rgb]{ .949,  .949,  .949}10 & \cellcolor[rgb]{ .949,  .949,  .949}7 & \cellcolor[rgb]{ .949,  .949,  .949}0.32 & \cellcolor[rgb]{ .949,  .949,  .949}0.03 & \cellcolor[rgb]{ .949,  .949,  .949}44.93 & \cellcolor[rgb]{ .949,  .949,  .949}14.98 & \cellcolor[rgb]{ .949,  .949,  .949}60.07 \\
              & AC11  & UNK   & UNK   & UNK   & 9     & 0.00  & 0     & 0     & 9     & 9     & 0     & 0.12  & 0.04  & 100.15 & 100.13 & 200.73 \\
              & \cellcolor[rgb]{ .949,  .949,  .949}AC12 & \cellcolor[rgb]{ .949,  .949,  .949}UNK & \cellcolor[rgb]{ .949,  .949,  .949}UNK & \cellcolor[rgb]{ .949,  .949,  .949}UNK & \cellcolor[rgb]{ .949,  .949,  .949}21 & \cellcolor[rgb]{ .949,  .949,  .949}0.08 & \cellcolor[rgb]{ .949,  .949,  .949}0 & \cellcolor[rgb]{ .949,  .949,  .949}12 & \cellcolor[rgb]{ .949,  .949,  .949}9 & \cellcolor[rgb]{ .949,  .949,  .949}9 & \cellcolor[rgb]{ .949,  .949,  .949}0 & \cellcolor[rgb]{ .949,  .949,  .949}0.34 & \cellcolor[rgb]{ .949,  .949,  .949}0.01 & \cellcolor[rgb]{ .949,  .949,  .949}44.90 & \cellcolor[rgb]{ .949,  .949,  .949}42.91 & \cellcolor[rgb]{ .949,  .949,  .949}88.07 \\
      \hline
\end{tabular}%
\label{tab:utility-appendix}%
\end{table*}%
